# Supplementary material for: Characterizing and Forecasting User Engagement with In-app Action Graph: A Case Study of Snapchat
Source: arXiv:1906.00355 source file (2019-06-02)
Supplement: Supplementary file 1 [file appendix.tex]

\appendix
\section{Common Path Tables}

%top patterns table
\begin{table}[h]
\tiny
\caption{Top 2-hop paths}
\label{tab: top 2-hop patterns}
\begin{tabular}{|ll|}
\hline
1&$CHAT\_VIEW \rightarrow CHAT\_SEND \rightarrow CHAT\_VIEW$   \\
2&$CHAT\_SEND \rightarrow CHAT\_VIEW \rightarrow CHAT\_SEND$   \\
3&$SNAP\_VIEW \rightarrow SNAP\_CREATE \rightarrow SNAP\_SEND$ \\
4&$SESSION\_START \rightarrow CHAT\_VIEW \rightarrow CHAT\_SEND$ \\
5&$CHAT\_VIEW \rightarrow CHAT\_SEND \rightarrow SESSION\_END$ \\
6&$SNAP\_CREATE \rightarrow SNAP\_SEND \rightarrow SESSION\_END$   \\
7&$SNAP\_CREATE \rightarrow SNAP\_SEND \rightarrow SNAP\_VIEW$   \\
8&$SESSION\_START \rightarrow SNAP\_VIEW \rightarrow SNAP\_CREATE$ \\ 
9&$SNAP\_SEND \rightarrow SNAP\_VIEW \rightarrow SNAP\_CREATE$ \\ 
10&$SESSION\_START \rightarrow STORY\_VIEW \rightarrow SESSION\_END$ \\ 
11&$CHAT\_VIEW \rightarrow CHAT\_SEND \rightarrow STORY\_VIEW$   \\
12&$SNAP\_CREATE \rightarrow SNAP\_SEND \rightarrow SNAP\_CREATE$   \\
13&$SNAP\_SEND \rightarrow SNAP\_CREATE \rightarrow SNAP\_SEND$   \\
14&$SNAP\_CREATE \rightarrow SNAP\_SAVE \rightarrow SNAP\_CREATE$   \\
15&$CHAT\_VIEW \rightarrow CHAT\_SEND \rightarrow SNAP\_VIEW$   \\
16&$STORY\_VIEW \rightarrow CHAT\_VIEW \rightarrow CHAT\_SEND$   \\
17&$SNAP\_SAVE \rightarrow SNAP\_CREATE \rightarrow SNAP\_SAVE$   \\
18&$SESSION\_START \rightarrow CHAT\_VIEW \rightarrow SESSION\_END$ \\ 
19&$SNAP\_CREATE \rightarrow SNAP\_SEND \rightarrow STORY\_VIEW$  \\
20&$SESSION\_START \rightarrow CHAT\_SEND \rightarrow SESSION\_END$ \\  \hline
\end{tabular}
\end{table}

\begin{table}[h]
\tiny
\caption{Top 1-hop paths}
\label{tab: top 1-hop patterns}
\begin{tabular}{|ll|}
\hline
1&$CHAT\_VIEW \rightarrow CHAT\_SEND$   \\
2&$CHAT\_SEND \rightarrow CHAT\_VIEWD$   \\
3&$SNAP\_CREATE \rightarrow SNAP\_SEND$ \\
4&$SESSION\_START \rightarrow CHAT\_VIEW$ \\
5&$SNAP\_VIEW \rightarrow SNAP\_CREATE$\\
6&$CHAT\_SEND \rightarrow SESSION\_END$ \\
7&$SESSION\_START \rightarrow SNAP\_VIEW$ \\ 
8&$STORY\_VIEW \rightarrow SESSION\_END$   \\
9&$SNAP\_SEND \rightarrow SESSION\_END$   \\
10&$SESSION\_START \rightarrow STORY\_VIEW$ \\
11&$SESSION\_START \rightarrow SNAP\_CREATE$ \\
12&$SNAP\_SEND \rightarrow SNAP\_VIEW$ \\
13&$CHAT\_SEND \rightarrow STORY\_VIEW$ \\
14&$SNAP\_CREATE \rightarrow SNAP\_SAVE$\\
15&$SNAP\_SEND \rightarrow SNAP\_CREATE$\\
16&$CHAT\_VIEW \rightarrow SESSION\_END$ \\
17&$CHAT\_SEND \rightarrow SNAP\_VIEW$ \\
18&$SESSION\_START \rightarrow CHAT\_SEND$ \\
19&$SNAP\_CREATE \rightarrow SESSION\_END$\\
20&$SNAP\_VIEW \rightarrow SESSION\_END$\\  \hline
\end{tabular}
\end{table}
